# Supplementary material for: Barrier and penalty methods for low-rank semidefinite programming with application to truss topology design
Source: arXiv:2105.08529 source file (2021-05-18)
Supplement: Supplementary file 1 [file appendix.tex]

\section*{Appendix} \label{sec:appendix}

{\color{red}MK: Included here are some results that I wasn't sure where to put:}

\begin{Lemma}
Let $X\in \S^n$ such that $\rank X = k$, $k\leq n$. Then $\rank (X\otimes X) = k^2$.
\end{Lemma}
\begin{Proof}
{\color{red}MK:Well known and easy to prove.}
\end{Proof}

\begin{Lemma}
Let $Y\in \S^n$ such that $\rank Y = k$, $k\leq n$, and $A\in\RR^{m\times n}$, $m<n$. Then $\rank(AYA^T)\leq k$.
\end{Lemma}
\begin{Proof}
Because $\rank Y = k$, we have $Y=\sum_{i=1}^k y^{(i)}(y^{(i)})^T$ with some $y^{(i)}\in\RR^n$, $i=1,\ldots,k$. Hence $AYA^T = A\left(\sum_{i=1}^k y^{(i)}(y^{(i)})^T\right)A^T = \sum_{i=1}^k z^{(i)}(z^{(i)})^T$ with $z^{(i)}=Ay^{(i)}$. Therefore $\rank (AYA^T)=\rank\sum_{i=1}^k z^{(i)}(z^{(i)})^T \leq k$.\\ {\color{red}MK: Explain why it can be smaller than k.}
\end{Proof}

\begin{Corollary}
Let $W$ be the scaling matrix from the IP part and let $\rank W = k$. Then $\rank H \leq\ k^2$, where $H$ is the Schur complement matrix from equation...
\end{Corollary}

{\color{red}MK: WHY IS THE IDEA OF ZHANG-LAVAEI PAPER BASICALLY FLAWED}

Zhang-Lavaei paper assumes that 
$$ W = W_0 +UU^T$$
where $\kappa(W_0)\in O(1)$ and $\rank U \leq k$, $k$ small.

This assumption, together with the Corollary above, means that $H$ has $k^2$ outlying eigenvalues and the rest goes \emph{uniformly} to zero ($W_0$ is well-conditioned and tends to zero matrix). This, however, means that the CG method \emph{without any preconditioning} needs $k^2$ iterations to significantly reduce the error, see the proposition below. Assuming that $k$ is very small, this means that we don't need a preconditioner. So, \emph{for problems satisfying Zhang-Lavaei assumption, we can use CG without preconditioning.} This is also confirmed by numerical examples when no preconditioner version needs about the same number of CG iterations (perhaps slightly more) but is far more efficient than any preconditionr CPU time-wise.

\medskip
The next proposition \cite[p.53]{cg} shows error reduction in the $i$-th iterate of CG for matrices with $k$ outlying eigenvalues.
\begin{Proposition}
	Given $x^0,b\in \mathbb{R}^n$, $A\in \mathbb{S}_{++}^n$, define $x^*=A^{-1}b$. 
	Assume that $A$ has $k$ large outlying eigenvalues:
	$$
	    \lambda_1(A)\leq\cdots\leq\lambda_{n-k}\ll \lambda_{n-k+1}\leq\cdots\lambda_n\,,
	$$
	where $k\ll n$.
	Then the $i$-th iterate of CG satisfies
	\begin{align}
	\label{cg}
	\frac{\|x^i-x^*\|}{\|x^0-x^*\|}\leq 2 \left(\frac{\sqrt{\kappa_{n-k}}-1}{\sqrt{\kappa_{n-k}}+1}\right)^{i-j}
	\end{align}
	with $\kappa_{n-k}=\lambda_{n-k}(A)/\lambda_{1}(A)$.
\end{Proposition}
In other words, the behaviour of CG for matrices with $k$ large outlying eigenvalues is determined by the distribution of the first $n-k$ eigenvalues. {\color{red}MK: This proposition is also cited by Zhang-Lavaei.}
